# Supplementary material for: Guided Statistical Workflows with Interactive Explanations and Assumption Checking
Source: arXiv:2410.00365 source file (2024-10-01)
Supplement: Supplementary file 1 [file 08_appendix.tex]

% \appendix 

% Appendix
